# Supplementary material for: Mixture representations and Bayesian nonparametric inference for likelihood ratio ordered distributions
Source: arXiv:2110.04852 source file (2023-10-26)
Supplement: Supplementary file 1 [file NotesOnAdditionalApplications.tex]

%We briefly sketch a semi-parametric approach along the lines of \citet{Sun1997} or \citet{Lee2001}. As in those articles, we can assume $g$ belongs to a parametric family indexed by a parameter $\vartheta$ while treating the monotonic weight function $w$ nonparametrically. For concreteness, suppose that $w$ is non-increasing. If the conditions of Theorem \ref{thm:fmixture_ac} are met, the mixture representation \eqref{fx_mixture} exists, and we can make inferences regarding $(\vartheta, u, \theta)$ and, in turn, the weight function $w$ from the observed data. Our sketch omits important theoretical and practical details, but further illustrates the range of problems to which statistical methods for likelihood ratio ordered distributions can be applied. 



%omitting many important details

%To avoid identifiability issues, we assume $g$ belongs to a parametric family, but treat the monotonic weight function $w$ nonparametrically. We could do the same.  Under a few additional assumptions, the mixture representation \eqref{fx_mixture} exists. We can estimate 

%Suppose that $g$ belongs to a parametric family indexed by a parameter $\vartheta$ and then  


%\citet{Sun1997} and \citet{Lee2001} suppose that 


%Following the semi-parametric approach of \citet{Sun1997} and \citet{Lee2001}, we could suppose that $g$ belongs to a parametric family indexed by a parameter $\vartheta$ and then  

%For example, suppose the weight function $w$ is non-increasing and $g$ belongs to a parametric family indexed by a parameter $\vartheta.$ Then 


%Suppose we expect the weight function $w$ to be non-increasing. We could, as in \citet{Sun1997} or \citet{Lee2001}, take a semi-parametric approach to the problem by assuming $g$ belongs to a parametric family indexed by a parameter $\vartheta.$
 
%Suppose that $w$ is non-increasing and locally absolutely continuous. We could, as in \citet{Sun1997} or \citet{Lee2001}, take a semi-parametric approach to the problem by supposing $g$ belongs to a parametric family. Then 


%and density estimation with a likelihood ratio constraint can be brought to bear on the problem of selection bias.

\iffalse
\begin{itemize}    
    \item %Inference for likelihood ratio ordered probability distributions is closely connected to shape-constrained inference for the receiver operating characteristic (ROC) curve, the area under the curve (AUC), and the probability $\text{pr}(X < Y)$ where $X \sim F$ and $Y \sim G$ are independent. 
    The receiver operating characteristic curve \citep{Pepe2004} describes the performance of a diagnostic test constructed from a continuous variable. % in terms of the true positive rate and false positive rate at each possible threshold. 
    Suppose, for example, that $F$ and $G$ are the distributions of a particular biomarker in healthy and diseased individuals, respectively. A cutoff $c$ is chosen and individuals with a score greater than $c$ receive a positive diagnosis. %he others receive a negative diagnosis.  %The ROC curve is defined by the map which sends $t \mapsto \left\{t, 1-G\left[F^{-1}(1-t)\right]\right\}$ for $t\in [0,1].$ 
    The receiver operating characteristic curve is traced out by plotting the true positive rate $1-G(c)$ against the false positive rate $F(c)$ for every possible choice of cutoff. %as the threshold $t$ varies from $-\infty$ to $\infty.$
    Equivalently, one can plot $\text{ROC}(t) = 1 - G\left\{F^{-1}(1-t)\right\}$ against $t$ for $t \in [0,1].$ The area under the curve is defined as $\text{AUC}(t) = \int_0^1 \text{ROC}(t) \, dt$ and is equal to $\text{P}(X < Y)$ where $X \sim F$ and $Y \sim G$ are independent. This quantity is of interest in medicine, engineering, and other fields as an intuitive measure of diagnostic performance \citep{Pepe2004}, treatment effectiveness \citep{Wolfe1971}, and component reliability \citep{Johnson1988, Kotz2003}. Estimating the receiver operating characteristic curve \citep{Hsieh1996, Zou1997, Lloyd1998,  Qin2003, Wan2007, Gu2008, Hanson2008, Zhu2020}, area under the curve \citep{Faraggi2002, Wang2020}, and $\text{pr}(X < Y)$ \citep{Enis1971, Zhou2008, Ventura2011, Rubio2013} are all active areas of research with literatures too vast to survey exhaustively. Importantly, the receiver operating characteristic curve is concave when $F \leq_{\text{LR}} G$ \citep{Hsieh1996}. \citet{Yu2017} describe how the quite natural problem of concave receiver operating characteristic curve estimation, considered by \citet{Lloyd200,Lloyd2002}, can be addressed via density estimation with a likelihood ratio order constraint. 
    
    \item Accounting for selection bias is a central problem in statistics. The problem is often formulated as follows. We aim to estimate the density function $f$ associated with a random variable $X.$ However, we only observe $X$ with probability $w(X).$ The conditional density of $X,$ given that it is observed, is then $g(x) \propto w(x) f(x).$ The function $w$ is called the ``biasing" or ``weight" function. In many applications, we expect the weight function $w$ to be monotone \citep{Sun1997, Lee2001}. For example, consider wildlife population data collected through an aerial census \citep{Cook1974}. We would expect that the probability of observing a group of animals from an airplane increases monotonically with the size of the group. In meta-analysis, we would expect that studies with small p-values have a higher probability of being published than those with large p-values \citep{Bayarri1987, Iyengar1988, Silliman1997, Silliman1997a}. The monotone weight function $w(x) \propto x$ gives rise to ``size-biased" or ``length-biased" data \citep{Cox1969, Patil1978}. When $w$ is monotone, the ratio $f/g$ is monotone and, potentially, density estimation with a likelihood ratio constraint can be brought to bear on the problem of selection bias.
    
    \item Poisson processes. Examples: Whether a particular adverse event is becoming more common as efforts are made to reduce another type. Whether citations of a particular method decrease as another becomes ascendant. 
    
\end{itemize}
\fi 
